# Supplementary material for: Exploring the Value of Pre-trained Language Models for Clinical Named Entity Recognition
Source: arXiv:2210.12770 source file (2023-10-30)
Supplement: Supplementary file 1 [file Appendices.tex]

\label{appendix}
We list the confusion matrices from each of the model evaluation, detailed BIOES level evaluation scores, as well as the scores from different batch size settings.

%\section*{Appendix A: other parameter/model settings}

\section*{Appendix-A: Confusion Matrix}
We report the confusion matrices from three different models on how they mis-label each of the nine classes and on overall binary evaluation in Figure \ref{fig:BioformerApt_confusion_token_all_classes} and \ref{fig:BioformerApt_confusion_token_binary} for BioformerApt, Figure \ref{fig:TransformerCRF_confusion_token_all_classes} and \ref{fig:TransformerCRF_confusion_token_binary} for TransformerCRF (BioformerCRF having very similar score to TransformerCRF). %xx xx and xx.

%\subsection*{A1: BioformerApt Confusion Matrix}

%\begin{figure*}[!t]
\begin{figure}[!t]
\begin{center}
\centering
\includegraphics*[width=0.49\textwidth]{./figs/bioformerApt_confusion_matrix_for_epoch_0001_in_test_token_evaluation}
\caption{BioformerApt Confusion matrix at token level evaluation from Epoch 1.}
\label{fig:BioformerApt_confusion_token_all_classes}
\end{center}
\end{figure}

%\begin{figure*}[!t]
\begin{figure}[!t]
\begin{center}
\centering
\includegraphics*[width=0.49\textwidth]{./figs/bioformerApt_confusion_matrix_for_epoch_0001_in_test_binary_evaluation}
\caption{BioformerApt Confusion matrix for binary evaluation at token level from Epoch 1.}
\label{fig:BioformerApt_confusion_token_binary}
\end{center}
\end{figure}

%\subsection*{A2: TransformerCRF Confusion Matrix}

%\begin{figure*}[!t]
\begin{figure}[!t]
\begin{center}
\centering
\includegraphics*[width=0.49\textwidth]{./figs/TranCRF_confusion_matrix_for_epoch_0008_in_test_token_evaluation}
\caption{TransformerCRF Confusion matrix at token level evaluation from Epoch 8.}
\label{fig:TransformerCRF_confusion_token_all_classes}
\end{center}
\end{figure}

%\begin{figure*}[!t]
\begin{figure}[!t]
\begin{center}
\centering
\includegraphics*[width=0.49\textwidth]{./figs/TranCRF_confusion_matrix_for_epoch_0008_in_test_binary_evaluation}
\caption{TransformerCRF Confusion matrix for binary evaluation at token level from Epoch 8.}
\label{fig:TransformerCRF_confusion_token_binary}
\end{center}
\end{figure}

\begin{comment}
\subsection*{A3: BioformerCRF Confusion Matrix}

%\begin{figure*}[!t]
\begin{figure}[!t]
\begin{center}
\centering
\includegraphics*[width=0.49\textwidth]{./figs/BiofCRF_confusion_matrix_for_epoch_0010_in_test_token_evaluation}
\caption{BioformerCRF Confusion matrix at token level evaluation from Epoch 10.}
\label{fig:BioformerCRF_confusion_token_all_classes}
\end{center}
\end{figure}

%\begin{figure*}[!t]
\begin{figure}[!t]
\begin{center}
\centering
\includegraphics*[width=0.49\textwidth]{./figs/BiofCRF_confusion_matrix_for_epoch_0010_in_test_binary_evaluation}
\caption{BioformerCRF Confusion matrix for binary evaluation at token level from Epoch 10.}
\label{fig:BioformerCRF_confusion_token_binary}
\end{center}
\end{figure}

\end{comment}

\section*{Appendix-B: BIOES Level Scores}

%\begin{figure*}[!t]
\begin{figure}[!t]
\begin{center}
\centering
\includegraphics*[width=0.49\textwidth]{./figs/BiofApt_classification_report_for_epoch_0001_in_test_bio_evaluation}
\caption{BioformerApt classification report for all BIOES sub-classes at Epoch 1.}
\label{fig:BioformerApt_classification_bioes}
\end{center}
\end{figure}

The BIOES level of classification report from BioformerApt is shown in Figure \ref{fig:BioformerApt_classification_bioes}. The BIOES level classification report of TransformerCRF and BioformerCRF mostly only fused on S-Drug and S-strength two sub-classes.

\section*{Appendix-C: Batch Size Matters}

We report more experimental results from different batch size settings and the findings show that batch size difference does make an influence on model performances. This can be related to our model settings or the very limited of amount of constrained training data from n2c2 shared task. % on our designed models.

Figure \ref{fig:BioformerApt_bs10_f1_score} and \ref{fig:BioformerCRF_bs10_f1_score} show the F1 score learning curves from BioformerApt and BioformerCRF at batch size 10. Figure \ref{fig:TransformerCRF_bs1_f1_score} and \ref{fig:BioformerCRF_bs1_f1_score} show the F1 score learning curves from TransformerCRF and BioformerCRF at batch size 1.

%\begin{figure*}[!t]
\begin{figure}[!t]
\begin{center}
\centering
\includegraphics*[width=0.49\textwidth]{./figs/BioformerApt_bs10_f1_score_vs_epoch_for_all_classes}
\caption{BioformerApt F1 score with each epoch for all classes with batch size as 10.}
\label{fig:BioformerApt_bs10_f1_score}
\end{center}
\end{figure}

%\begin{figure*}[!t]
\begin{figure}[!t]
\begin{center}
\centering
\includegraphics*[width=0.49\textwidth]{./figs/BioformerCRF_bs10_f1_score_vs_epoch_for_all_classes}
\caption{BioformerCRF F1 score with each epoch for all classes with batch size as 10.}
\label{fig:BioformerCRF_bs10_f1_score}
\end{center}
\end{figure}

%\begin{figure*}[!t]
\begin{figure}[!t]
\begin{center}
\centering
\includegraphics*[width=0.49\textwidth]{./figs/TranCRF_bs1_f1_score_vs_epoch_for_all_classes}
\caption{TransformerCRF F1 score with each epoch for all classes with batch size as 1.}
\label{fig:TransformerCRF_bs1_f1_score}
\end{center}
\end{figure}

%\begin{figure*}[!t]
\begin{figure}[!t]
\begin{center}
\centering
\includegraphics*[width=0.49\textwidth]{./figs/BioformerCRF_bs1_f1_score_vs_epoch_for_all_classes}
\caption{BioformerCRF F1 score with each epoch for all classes with batch size as 1.}
\label{fig:BioformerCRF_bs1_f1_score}
\end{center}
\end{figure}

\section*{Appendix-D: Deploying ClinicalBERT}
\subsection*{ClinicalBERT-CRF}
We also deployed Clinical-BERT (ClinicalBERT) \cite{alsentzer-etal-2019-publicly_bioclinicalBERT} which was fine-tuned from BioBERT using MIMIC clinical data such as discharged summaries \footnote{model available at \url{https://github.com/EmilyAlsentzer/clinicalBERT}}. We applied CRF layer on top of ClinicalBERT for our experiments. However, the evaluation results do not show much difference/improvement from BioformerCRF (pre-trained plus fine-tuning) and TransformerCRF (learned from 300 letters only). We believe this is related to difficulty of this challenge task itself, e.g. the nine categories of special tokens and their very low frequencies in the context. 
The total trainable parameters for ClinicalBERT-CRF is 108,311,793 which is 3.07 times of TransformerCRF (35,273,750) and 2.5 times of BioformerCRF (42,543,638).

\subsection*{ClinicalBERT-Apt}
We also tested the ClinicalBERT-Apt model, which removes our CRF layer but keeping an adaptation layer on top of ClinicalBERT \cite{alsentzer-etal-2019-publicly_bioclinicalBERT} (batch size = 4, \textit{ref.} setting at Section \ref{sub_sec_corpus_model_setting}). The performance is similar to BioformerApt just with slightly better F1 scores (0.90\% vs 0.69\%) and Corr (2086 \textit{vs} 1615) as in Table \ref{tab:CliBertApt_eval} from Epoch 1. This difference tells that the pre-training  corpus does have an effect, e.g. biomedical \textit{vs} clinical domains. However, from the 2nd epoch on-wards, it shows similar tendency with BioformerApt, i.e. much lower overall Accuracy scores, around 12.00\%, and mostly predicting/generating ADE labels.  
The total parameters and also the trainable parameters of ClinicalBERT-Apt is 108,310,272 which is bigger than BioformerApt which was 42,523,136.

\begin{table}[!t]
\begin{center}
\centering
\begin{tabular}{crccc}
\toprule
\multicolumn{1}{c}{Acc} 
     & \multicolumn{1}{c}{Pre }     
                & Rec   & F1   & Corr \\
\midrule
18.65 \% & 0.49\%    & 5.95\% & 0.90\% & 2086    \\
\hline
\multicolumn{1}{c}{Catergory} 
     & \multicolumn{1}{c}{Pre }     
                & Rec   & F1   & found \\
\midrule
ADE & 0.07\%    & 5.71\% & 0.14\% & 51759     \\
Dosage & 0.15\%    & 2.65\% & 0.28\% & 52284    \\ 
Drug & 1.92\%   & 9.46\%  & 3.19\% & 53833 \\ 
Duration & 0.01\%    & 1.46\% & 0.02\% & 51066   \\ 
Form & 0.45\%    & 4.82\% & 0.83\% & 48682 \\  
Frequency & 0.57\%    & 5.34\% & 1.04\% & 46571 \\  
Reason & 0.36\%    & 5.91\% & 0.67\% & 45147 \\  
Route & 0.60\%    & 7.04\% & 1.11\% & 41249 \\  
Strength & 0.09\% & 0.81\% & 0.16\% & 38777   \\  
\bottomrule
\end{tabular}
\caption{ClinicalBERT-Apt evaluation results using PLM ClinicalBERT with an adaptation layer. 
%Overall Accuracy, Precision, Recall, F1, and Correct tagging scores, and on each category. Trainable parameters: 42,523,136. Much lower overall acc scores though increased corr. much larger parameters than TransformerCRF and used large amount of pre-training data.
}
\label{tab:CliBertApt_eval}
\end{center}
\end{table}

\section*{Appendix-E: The Open Source Project}
Currently, our open-source project \url{https://github.com/poethan/TransformerCRF} hosts the following models which are available. 

\begin{itemize}
    \item TransformerCRF: word level model training from scratch
    \item BioformerCRF: PLM Bioformer with CRF fine-tuning
    \item BioformerApt: Using pre-trained parameters from Bioformer with an adaptation layer for text mining task
    \item ClinicalBERT-CRF: using pre-trained ClinicalBERT with CRF layer for fine-tuning
    \item ClinicalBERT-Apt: ClinicalBERT \cite{alsentzer-etal-2019-publicly_bioclinicalBERT} with adaptation layer
\end{itemize}

In the future, we plan to carry out the follow-up models using clinical domain pre-trained word embeddings together with sub-word / character-level learning.

The model dependencies/requirements include:

\begin{itemize}
    \item Python 3.7.13
    \item Tensorflow 1.14.0 / 2.9.1 (using 2.9.1)
    \item tensorflow-addons 0.17.0 (if use tf2)
    \item transformers 4.20.1
    \item matplotlib
    \item sklearn
    \item spacy
    \item pytorch
\end{itemize}

%We acknowledge the usage of the following packages: NeuroNER, Transformers, conll2003 eval shared task, Stanford coreNLP, Bioformer and ClinicalBERT.

\begin{comment}
%the difference made by these two different strategies:

\subsection{Word Embedding learned in-domain}
PWE with MIMIC-iii data plus TransformerCRF

\subsection{PLM using in-domain data}

using PLM Bio-ClinicalBERT \cite{alsentzer-etal-2019-publicly_bioclinicalBERT}:

Model-I:
Bio-ClinicalBERT / Bio-DischargedSummaryBERT -> with Positional encoding -> add and drop -> TransformerCRF
V1. shared positional encoding using the same one encoded via PLM
V2. continuously positional encoding to relearn it 

Model-II:
Bio-ClinicalBERT -> TransformerCRF

Model-III:
PLM -> classification layer + CRF (different with their original paper that applied to i2b2 data who only used classification layer afterwards ?)

Model-IV:
shall we set up a baseline that uses the original structure: PLM -> classification layer? 

\subsubsection{ClinicalBERT-CRF}

Surprisingly, after 15 epochs using batch size 4, the ClinicalBERT-CRF has almost the same scores as our TransformerCRF

\end{comment}
